# Supplementary material for: Semantic Complete Scene Forecasting from a 4D Dynamic Point Cloud Sequence
Source: arXiv:2312.08054 source file (2023-12-15)
Supplement: Supplementary file 1 [file results_supp.tex]

\newcommand{\tablestyle}[2]{\setlength{\tabcolsep}{#1}\renewcommand{\arraystretch}{#2}\centering\footnotesize}
\newcolumntype{Y}{>{\centering\arraybackslash}X}

\begin{table}[t]
\centering
\footnotesize
\tablestyle{2.5pt}{1.05}
\begin{tabularx}{1.0\linewidth}{lY|YYY}
    \toprule
    \multicolumn{1}{c}{Task} & \multicolumn{1}{c}{Prediction} & \multicolumn{3}{c}{Complete Prediction} \\
     & CD & CD & IOU & mIOU \\
    \midrule
    TLFPAD \cite{tlfpad} & 0.043 & - & - & - \\ %
    Occlusion4D(SF) \cite{vanhoorick2022revealing} & 0.050 & - & - & - \\ %
    Occlusion4D(CSF) \cite{vanhoorick2022revealing} &0.255 & 0.129 & - & - \\ %
    Occlusion4D(SCSF) \cite{vanhoorick2022revealing} & 0.185 & 0.093 & 23.0(11.6) & 12.7(7.4) \\ %
    \hline
    SF & 0.051 & - & - & - \\
    CSF & 0.039 & 0.032 & 42.3(26.6) & - \\
    SCSF & 0.038 & 0.032 & 42.6(31.0) & 31.2(22.4) \\
    \bottomrule
\end{tabularx}
\vspace{-0.1cm}
\caption{\textbf{Results on IGPLAY dataset}. We report Chamfer Distance of point clouds(lower is better, the unit is square meter), IoU of low-resolution voxel grids(on the left) as well as high-resolution ones(on the right, in brackets), and mIoU of low-resolution voxel grids(on the left) as well as high-resolution ones(on the right, in brackets).}
\vspace{-0.3cm}
\label{tables:igplay_sup}
\end{table}

\setlength{\tabcolsep}{2pt}

\begin{table}[t]
\centering
\footnotesize
\tablestyle{2.5pt}{1.05}
\begin{tabularx}{1.0\linewidth}{lY|YYY}
    \toprule
    \multicolumn{1}{c}{Task} & \multicolumn{1}{c}{Prediction} & \multicolumn{3}{c}{Complete Prediction} \\
     & CD & CD & IOU & mIOU \\
    \midrule
    TLFPAD \cite{tlfpad} & 0.047 & - & - & - \\ %
    Occlusion4D(SF) \cite{vanhoorick2022revealing} & 0.100 & - & - & - \\ %
    Occlusion4D(CSF) \cite{vanhoorick2022revealing} & 0.200 & 0.113 & - & - \\ %
    Occlusion4D(SCSF) \cite{vanhoorick2022revealing} & 0.190 & 0.138 & 49.2(41.3) & 23.5(18.9) \\ %
    \hline
    SF & 0.038 & - & - & - \\
    CSF & 0.034 & 0.028 & 66.8(50.2) & - \\
    SCSF & 0.030 & 0.023 & 69.1(54.9) & 33.7(27.6) \\
    \bottomrule
\end{tabularx}
\vspace{-0.1cm}
\caption{\textbf{Results on IGNAV dataset}. We report Chamfer Distance of point clouds(lower is better, the unit is square meter), IoU of low-resolution voxel grids(on the left) as well as high-resolution ones(on the right, in brackets), and mIoU of low-resolution voxel grids(on the left) as well as high-resolution ones(on the right, in brackets).}\vspace{-0.4cm}
\label{tables:ignav_sup}
\end{table}
