# Supplementary material for: Semantic Complete Scene Forecasting from a 4D Dynamic Point Cloud Sequence
Source: arXiv:2312.08054 source file (2023-12-15)
Supplement: Supplementary file 2 [file ablations_supp.tex]

\newcolumntype{Y}{>{\centering\arraybackslash}X}

\begin{table}[t]
\centering
\footnotesize
% \tablestyle{2.5pt}{1.05}
\begin{tabularx}{1.0\linewidth}{lYYYY}
    \toprule
    \multicolumn{1}{c}{Task} & \multicolumn{1}{c}{CD(surf.)} & \multicolumn{1}{c}{CD(cmpl.)} & \multicolumn{1}{c}{IoU} & \multicolumn{1}{c}{mIoU} \\
    \midrule
    no implicit & 0.734 & 0.655 & 44.6~(14.4) & 32.1~(10.8) \\ %
    % with true mask & - & - & 47.2~(30.6) & 33.6~(22.1) \\
    no  visibility grid & 0.051 & 0.042 & 43.2~(30.6) & 27.6~(20.3) \\
    no cross-attention & 0.062 & 0.045 & 37.8~(26.9) & 28.3~(20.5) \\
    no dilated conv & 0.065 & 0.050 & 41.5~(24.4) & 29.8~(18.2) \\
    voxel encoder & 0.049 & 0.040 & 42.2~(30.1) & 28.2~(20.0) \\
    data augmentation & 0.037 & 0.032 & 46.1~(31.1) & 32.1~(22.6) \\
    Ours & 0.038 & 0.032 & 42.6~(31.0) & 31.2~(22.4) \\ %
    \bottomrule
\end{tabularx}
\vspace{-0.1cm}
\caption{\textbf{Ablation study of SCSFNet on IGPLAY dataset.} Here both IoU and mIoU are evaluated in both low-resolution(on the left) and high-resolution(on the right, in brackets) settings.}
\vspace{-0.3cm}
\label{tables:ablations_supp}
\end{table}

\setlength{\tabcolsep}{2pt}
